# Supplementary material for: Orbital Ordering in the Charge Density Wave Phases of BaNi$_2$(As$_{1-x}$P$_x$)$_2$
Source: arXiv:2509.05200 source file (2026-01-23)
Supplement: Supplementary file 1 [file SM.tex]

\documentclass[%
%reprint,
superscriptaddress,
%groupedaddress,
%unsortedaddress,
%runinaddress,
%frontmatterverbose, 
%preprint,
%preprintnumbers,
%nofootinbib,
%nobibnotes,
%bibnotes,
 amsmath,amssymb,
 aps,
%pra,
prl,
%rmp,
%prstab,
%prstper,
%floatfix,
]{revtex4-2}

\usepackage{graphicx}% Include figure files
\usepackage{dcolumn}% Align table columns on decimal point
\usepackage{bm}% bold math
\usepackage{makecell}
\usepackage{placeins}
%\usepackage{hyperref}% add hypertext capabilities
%\usepackage[mathlines]{lineno}% Enable numbering of text and display math
%\linenumbers\relax % Commence numbering lines

%\usepackage[showframe,%Uncomment any one of the following lines to test 
%%scale=0.7, marginratio={1:1, 2:3}, ignoreall,% default settings
%%text={7in,10in},centering,
%%margin=1.5in,
%%total={6.5in,8.75in}, top=1.2in, left=0.9in, includefoot,
%%height=10in,a5paper,hmargin={3cm,0.8in},
%]{geometry}

\usepackage{braket}

%Cross referencing
\usepackage{xr}
\usepackage[hidelinks]{hyperref}
%Actually "load" the SM
\externaldocument[Main:]{Main_aux}

%Load own packages
\usepackage{siunitx}
\DeclareSIUnit\angstrom{\text{Å}}
\DeclareSIUnit\bar{bar}
\usepackage[capitalise]{cleveref}

%For SM only

\usepackage{multirow}
\usepackage{tabularx}
\usepackage{placeins} %Defines a \FloatBarrier command, beyond which floats may not pass; useful, for example, to ensure all floats for a section appear before the next \section command. 

\begin{document}

\include{Definitions}
\title{Supplemental Material: \titlename}
\include{Authors}
\date{\today}% It is always \today, today,
             %  but any date may be explicitly specified
\maketitle

\section{Crystal Growth and samples}
BaNi$_2$(As$_{1-\mathrm{x}}$P$_\mathrm{x}$)$_2$ single crystals were grown using the self-flux method. First, NiAs was synthesized by mixing pure Ni powder (Alfa Aesar 99.999\%) with milled pure As lumps (Alfa Aesar 99.9999\%). The mixture was sealed under vacuum in a fused silica tube and annealed for \SI{20}{\hour} at \SI{730}{\celsius}.  For the final growth of BaNi$_2$(As$_{1-\mathrm{x}}$P$_\mathrm{x}$)$_2$ single crystals, a ratio of {Ba:NiAs:Ni:P = 1:4(1-x):4x:4x} was placed in an alumina or glassy carbon tube, which was sealed in an evacuated quartz ampule (i.e. \SI{1e-5}{\milli\bar}). All sample handling was performed in an argon glove box (O$_2$ content \SI{0.7}{ppm}). The mixtures were heated to \SIrange{500}{700}{\celsius} for \SI{10}{\hour}, followed by heating slowly to a temperature of \SIrange{1100}{1150}{\celsius}, soaked for \SI{5}{\hour}, and subsequently cooled to \SIrange{995}{950}{\celsius} at the rate of \SIrange{0.5}{1}{\celsius\per\hour}, depending on the phosphorus content used for the growth. At \SIrange{995}{950}{\celsius}, the furnace was canted to remove the excess flux, followed by furnace cooling. Plate-like single crystals with typical sizes \qtyproduct[product-units=power]{2 x 2 x 0.5}{\milli\metre} were easily removed from the remaining ingot. The crystals were brittle, with a shiny brass-yellow metallic luster. The substitution level was determined with energy dispersive x-ray spectroscopy (EDX) using a COXEM EM-30AXN SEM-EDX scanning electron microscope with an Oxford Instruments Aztec EDX system.

In the main text, results from three samples are discussed. Samples 1 and 2 are non-substituted samples. Sample 3 is phosphorus substituted with a phosphorus content of \(x\approx0.059 \pm 0.005\). Sample 1 is shown in \cref{Main:Fig:Geo+Sample}c,d in the main text and was measured at beamline UE46 PGM. Samples 2 and 3 were measured at beamline ID32. Here in the Supplemental material additional data from the non-substituted samples 4, 5 and 6 are presented. Samples 4 and 5 were measured at beamline UE46 PGM and were aligned with the \(c\)-axes being the surface normal. Sample 6 was measured at beamline ID32. A complete overview is also given in \cref{Tab:SAmpleOverview}.

\begin{table}
    \centering
    \caption{\label{Tab:SAmpleOverview} An overview of all the investigated samples is provided, including their substitution content, orientation, and the applied experimental technique.}
    \begin{tabular}{l ccccccc}
        &  Sample 1 & Sample 2 & Sample 3 & Sample 4 & Sample 5 &Sample 6 \\
    \hline
     \(x\)   &  0.0 & 0.0 & 0.059(5) & 0.0 & 0.0 & 0.0 \\
     Beamline & UE46 PGM & ID32 & ID32 & UE46 PGM & UE46 PGM & ID32\\
     Orientation & \makecell{\(b\)-normal (I-CDW)\\\(b\)-normal tilted by \ang{19.5} (C-CDW)} & \(b\)-normal & \(b\)-normal & \(c\)-normal & \(c\)-normal & \(b\)-normal \\
     Investigated peak & \makecell{\((0\ 0.28\ 0)\)\\and \((0\ \frac{1}{3}\ -\frac{1}{3})\)} &  \makecell{\((0\ 0.28\ 0)\)\\and \((0\ \frac{1}{3}\ -\frac{1}{3})\)} & \((0\ 0.28\ 0)\) & \((0\ 0.28\ 1)\) & \((0\ 0.28\ 1)\) & \((0\ \frac{1}{3}\ -\frac{1}{3})\)\\
     Technique & REXS & REXS and RIXS & REXS & REXS & REXS & RIXS \\
    
    \end{tabular}
\end{table}

\section{Resonant Elastic and Inelastic X-ray Scattering}

The REXS measurements were conducted at the XUV diffractometer at beamline UE46 PGM at BESSY II \cite{Weschke2018} and the RIXS end-station at beamline ID32 at the ESRF \cite{Brookes2018}. In addition, RIXS measurements were performed at the RIXS end-station at beamline ID32 at the ESRF.

The experiments were performed at the L\textsubscript{3} edge \((\approx \qty{853}{\eV} )\). To reach the I-CDW and C-CDW positions in resonance, the measurements must be performed on the \(ac\) or \(bc\) side of the sample. Due to the plate-like morphology of\bnap, this corresponds to an edge of the sample. Accordingly, the samples were mounted on a copper slab, in order to tilt them by \ang{90} and get the \(b\)-axis as the normal. In this geometry are the samples directly correctly oriented for an azimuthal rotation when investigating the I-CDW. For the C-CDW measurements, however, the sample must be pre-tilted by an additional \(\approx \ang{19.5}\) to make the C-CDW wavevector the normal vector in order to be able to make an azimuthal rotation. For the measurements this was achieved by an additional copper wedge (beamline UE46 PGM). The corresponding scattering geometries are shown in the main text in \cref{Main:Fig:Geo+Sample}. The azimuthal angle \(\varphi\) is chosen in such a way that \ang{0} corresponds to the \(bc\) plane being the horizontal/scattering plane. The samples were roughly aligned by eye. A better alignment was made using the \(\{0\ 1\ 1\}\)-Bragg peak and the CDW peaks. The samples were cleaved in air just before transferring the samples into the ultra-high vacuum (UHV) chamber. An in-vacuum cleaving on the side of the sample was not possible, but also not necessary.

At beamline UE46 PGM, the beam was focused to a spot of \qtyproduct{100 x 50}{\micro\meter}. If not stated otherwise, all measurements were performed at the resonance of the CDWs at \qty{852.8}{\eV}. Some alignment scans of the otherwise non-reachable Bragg peak were also performed out-of-resonance. Only linearly polarized light and the orientation of the linear polarization was changed during the experiment. The signal was measured using a silicon diode. All measurements, except for the energy dependence, were performed using an entrance slit of \qty{200}{\micro\meter}. For the energy dependence, an entrance slit of \qty{100}{\micro\meter} was used.

At beamline ID32, the beam was focused to a spot of \qtyproduct{5 x 2}{\micro\meter}. The X-ray energy was changed during the experiments, but if not stated otherwise, the incoming X-ray energy was chosen to be at the resonance of the two CDWs at \qty{852.8}{\eV}. Alignment scans of the Bragg peaks not reachable in resonance were also performed off-resonant. Only linearly polarized horizontal or vertical light was used. For the RIXS measurements, the entrance slit was closed to \qty{15}{\micro\meter}, resulting in an energy resolution of \(\approx \qty{32.5}{\milli\eV}\). For the REXS measurements, the entrance slit was opened to \qty{100}{\micro\meter} to increase the flux. The REXS measurements were performed using the small silicon diode instead of the spectrometer arm.

\section{Discussion of the tensor atomic form factor of the I-CDW and C-CDW}

\subsection{The tensor atomic form factor and measured intensity}

For the discussion of the REXS data the polarization dependence of the scattering intensity of the I-CDW and C-CDW must be interpreted. For X-ray scattering, it can commonly be assumed that the scattering processes of the different atoms are independent \cite{Dmitrienko2013}. In this so-called isolated-atom approximation, the atomic scattering amplitude can be expressed as
\begin{align}
    f(\vec{k},\vec{\epsilon},\vec{k}',\vec{\epsilon}') = - \frac{e^2}{mc^2} f_{jk}(\vec{k}',\vec{k}) \vec{\epsilon}'_j\vec{\epsilon}_k
\end{align}
using the tensor atomic form factor \(f_{jk}(\vec{k}',\vec{k})\) and the incoming and outgoing polarizations \(\vec{\epsilon}_k\) and \(\vec{\epsilon}'_j\), respectively. The polarization vectors can be decomposed into the vertical \(\vec{\epsilon}_{i,v}\) and horizontal \(\vec{\epsilon}_{i,h}\) polarization vectors for the incoming \(i\) and scattered beam \(s\). These polarization vectors are fixed by the scattering geometry sketched in \cref{Main:Fig:Geo+Sample}a and can be expressed as
\begin{align}
    \vec{\epsilon}_{i,v} &= \begin{pmatrix}
                            \cos(\varphi)\\
                            0 \\
                            \sin(\varphi)        
                        \end{pmatrix}
    \quad & \vec{\epsilon}_{s,v} &= \begin{pmatrix}
                            \cos(\varphi)\\
                            0 \\
                            \sin(\varphi)        
                        \end{pmatrix}\\
    \vec{\epsilon}_{i,h} &= \begin{pmatrix}
                            -\sin(\varphi)\cos(\alpha)\\
                            \sin(\alpha) \\
                            \cos(\varphi)\cos(\alpha)      
                        \end{pmatrix}
    \quad & \vec{\epsilon}_{i,h} &= \begin{pmatrix}
                            \sin(\varphi)\cos(\alpha)\\
                            \sin(\alpha) \\
                            -\cos(\varphi)\cos(\alpha)      
                        \end{pmatrix}
\end{align}
including the azimuthal angle \(\varphi\) and the angle between the incoming beam and the scattering vector \(\alpha\).  The angle \(\alpha\) can be calculated using \(\theta\) or \(2\theta\) via
\begin{align}
    \alpha  &=  \ang{90}-\theta \\
            &= \frac{\ang{180}-2\theta}{2} \ .
\end{align}
For the further discussion also the wave vectors of the incoming and outgoing beams are relevant. Those can be represented as 
\begin{align}
    \vec{k} &= \begin{pmatrix}
                            -\sin(\varphi)\sin(\alpha)\\
                            -\cos(\alpha) \\
                            \cos(\varphi)\sin(\alpha)      
                        \end{pmatrix}
    \quad & \vec{k}' &= \begin{pmatrix}
                            -\sin(\varphi)\sin(\alpha)\\
                            \cos(\alpha) \\
                            \cos(\varphi)\sin(\alpha)      
                        \end{pmatrix} \ . \label{Eq:WVDef}
\end{align}
In the case of the measurements with the wedge for the C-CDW, the polarization vectors and wave vectors must be transformed from the laboratory frame to the crystal frame, as the two are tilted because of the wedge angle. The transformation can be done using the rotation matrix
\begin{equation}
    \mathbf{R} = \begin{pmatrix}
        1 & 0 & 0\\
        0 & \cos(\beta) & sin(\beta)\\
        0 &-sin(\beta) & \cos(\beta)
    \end{pmatrix}
\end{equation}
which includes the angle of the wedge \(\beta\).

Following the work from \textcite{Blume1983,Blume1985,Blume1994} the atomic tensorial scattering form factor can be calculated using the perturbation Hamiltonian
\begin{equation}
   \begin{aligned}
    \mathcal{H}' = & \frac{e^2}{2mc^2} \sum_i \vec{A}^2(\vec{r}_i) - \frac{e}{mc} \sum_i \vec{p}_i  \cdot \vec{A}(\vec{r}_i)
     - \frac{e\hbar}{mc} \sum_i \vec{s}_i \cdot \nabla \times \vec{A}(\vec{r}_i) 
     - \frac{e^2\hbar}{2\left(mc^2\right)^2} \sum_i \vec{s}_i \cdot \left(\dot{\vec{A}}(\vec{r}_i) \times \vec{A}(\vec{r}_i)\right) \label{Theo:eq:XHamilton}
\end{aligned} 
\end{equation}
including the vector potential \(\vec{A}(\vec{r}_i)\), the momentum operator \(\vec{p}_i\), the spin \(\vec{s}_i\) and \(i\) describing the \(i^\mathrm{th}\) electron. Using Fermi's first golden rule, the tensor atomic form factor can be expressed as

\begin{equation}
    \begin{aligned}
        f_{jk}(\vec{k}',\vec{k}) = & \sum_{\ket{g}} P_g \Biggl\{  \Braket{g|\sum_i \exp{\left(i\vec{q}\cdot\vec{r}_i\right)}|g} \delta_{jk} \\
        & - i \frac{\hbar \omega}{mc^2} \Braket{g|\sum_i \exp{\left(i\vec{q}\cdot\vec{r}_i\right)}\left(-\frac{\left[\vec{q}\times \vec{p}_i\right]_l}{\hbar \vec{q}^2} A_{jkl} + s_l^i B_{jkl}\right)|g} \\
        & - \frac{1}{m} \sum_{\ket{n}} \frac{E_g-E_n}{\hbar\omega} \frac{\Braket{g|O_j^\dag(\vec{k}')|n}\Braket{n|O_j(\vec{k})|g}}{E_g-E_n+\hbar\omega-i\frac{\Gamma}{2}} \\
        & - \frac{1}{m} \sum_{\ket{n}} \frac{E_g-E_n}{\hbar\omega} \frac{\Braket{g|O_j^\dag(\vec{k}')|n}\Braket{n|O_j(\vec{k})|g}}{E_g-E_n-\hbar\omega} \Biggl\} \label{Theo:eq:atomicForm}
    \end{aligned}
\end{equation}
with the probability \(P_g\) of state \(\ket{g}\) being occupied, the tensors \(A_{jkl}\) and \(B_{jkl}\) describing the charge scattering associated with the spin and orbital momentum. Furthermore, the vector operator
\begin{equation}
    \vec{O}(\vec{k}) = \sum_i \exp\left(i \vec{k}\cdot\vec{r}_i\right)\left(\vec{p}_i-i\hbar\left[\vec{k} \times \vec{s}_i\right]\right)
\end{equation}
is included. For the experiment in resonance, only the third part describing the resonant part \(f^\mathrm{res}\) of the tensor atomic form factor is relevant. The resonant part of the tensor atomic form factor can be simplified by using the expansion of the exponential function
\begin{equation}
    \exp\left(i\vec{k}\vec{r}_i\right) \approx 1 + \vec{k}\vec{r}_i + \frac{1}{2} \left(i\vec{k}\vec{r}_i\right)^2 + \ldots \label{Eq:TensorAtomicFormMulipol}
\end{equation}
in the vector operator \(\vec{O}\). This results to an expansion of the resonant atomic form factor tensor into Cartesian tensors given by
\begin{equation}
 f_{jk}^\text{res} \cong \underbrace{D_{jk}}_{\text{dipole-dipole}} + \underbrace{\frac{i}{2} I_{jkl}k_l - \frac{i}{2} I_{kjl}k_l'}_{\text{dipole-quadrupole}} + \underbrace{\frac{1}{4} Q_{jlkm}k_mk_l'}_{\text{quadrupole-quadrupole}} + \ldots
\end{equation}
including the dipole-dipole 2\textsuperscript{nd} rank tensor \(\mathbf{D}\), the dipole-quadrupole 3\textsuperscript{rd} rank tensor \(\mathbf{I}\) and the quadrupole-quadrupole 4\textsuperscript{th} rank tensor \(\mathbf{Q}\) \cite{Dmitrienko2013}. The scattering intensity is then given by
\begin{equation}
I(\vec{k},\vec{k}',\vec{\epsilon},\vec{\epsilon}') \propto \left| \sum_{j,k} \epsilon_j'^{*}\epsilon_k D_{jk} + \frac{i}{2} \sum_{j,k,l} \epsilon_j'^{*}\epsilon_k \left( k_l I_{jkl}-k_k' I_{kjl} \right) + \frac{1}{4} \sum_{j,k,l,m} \epsilon_j'^{*}\epsilon_k k_l' k_m Q_{jklm}  \right|^2 = \left| \vec{\epsilon} \mathbf{f}^\mathrm{res} \vec{\epsilon}' \right|^2 \ .
\end{equation}

As the scattered polarization cannot be differentiated in this experiment, the measured intensity \(I\) is linear combination of the vertically and horizontally polarized scattering intensities given by
\begin{align}
    I_v &\propto \left| \vec{\epsilon}_{s,v}^* \mathbf{f}^\mathrm{res} \vec{\epsilon}_{i,v} \right |^2 +\left  | \vec{\epsilon}_{s,h}^* \mathbf{f}^\mathrm{res} \vec{\epsilon}_{i,v}\right|^2 \\
    I_h &\propto \left| \vec{\epsilon}_{s,v}^* \mathbf{f}^\mathrm{res} \vec{\epsilon}_{i,h} \right |^2 + \left | \vec{\epsilon}_{s,h}^* \mathbf{f}^\mathrm{res} \vec{\epsilon}_{i,h}\right|^2 
\end{align}
for the case of incoming vertical and horizontal polarization, respectively. Experimentally, it is more reliable to investigate the ratio of the intensities of incoming vertical and horizontal polarization, as this eliminates varying intensities through the azimuthal dependence emerging from, for example, small changes of the measurement spot or the morphology of the sample. Hence, the investigated quantity is
\begin{equation}
    \frac{I_v}{I_h} = \frac{\left| \vec{\epsilon}_{s,v}^* \mathbf{R}\mathbf{f}^\mathrm{res}\mathbf{R}^T \vec{\epsilon}_{i,v} \right |^2 + \left | \vec{\epsilon}_{s,h}^* \mathbf{R}\mathbf{f}^\mathrm{res}\mathbf{R}^T \vec{\epsilon}_{i,v}\right|^2}{\left| \vec{\epsilon}_{s,v}^* \mathbf{R}\mathbf{f}^\mathrm{res}\mathbf{R}^T \vec{\epsilon}_{i,h} \right |^2 + \left | \vec{\epsilon}_{s,h}^* \mathbf{R}\mathbf{f}^\mathrm{res}\mathbf{R}^T \vec{\epsilon}_{i,h}\right|^2} \label{ed:IntRatioFull}
\end{equation}
after including the rotation matrix needed for the investigations with scattering geometries using a wedge. Note that for the case for dipole-quadrupole and quadrupole-quadrupole tensors the wave vectors which enter must also be transformed with the rotation matrix in the crystal frame, as they are defined in \cref{Eq:WVDef} in the laboratory frame. Furthermore, in the investigated intensity ratio, the resonant part of the tensor atomic form factor \(\mathbf{f}^\mathrm{res}\) is only defined up to an complex number. As \bnap does not exhibit any magnetic ordering, we only have to consider charge scattering. For charge scattering the dipole-dipole tensor is symmetric \cite{Dmitrienko2013} leading to
\begin{align}
    D_{jk} = D_{kj} \ .
\end{align}

Also the dipole-quadrupole and quadrupole-quadrupole tensor must fulfill in this case additional symmetries which are explained in more detail by \textcite{Dmitrienko2013}. The symmetry of the dipole-quadrupole tensors given by
\begin{align}
    I_{jkl} = I_{jlk} \ .
\end{align}

It is also important to note that the dipole-quadrupole term is allowed only for point groups without an inversion center.  Since the quadrupole-quadrupole components are usually negligible and the tensor includes too many components for a reasonable fit, we will not discuss the quadrupole-quadrupole terms further.

\subsection{I-CDW tensor atomic form factor: orthorhombic symmetry}

\textcite{Merz2021} find, based on available data, that the average crystal structure in the I-CDW phase is most likely of orthorhombic \textit{Immm} symmetry. In this structure, the nickel is at a 4j position resulting in a local symmetry at the nickel position of \textit{mm}2. The shape of the tensors is tabulated for all possible point groups and given by
\begin{align}
    \mathbf{D}_\mathrm{orth} &= \begin{pmatrix}
        D_{11} & 0 & 0\\
        0 & D_{22} & 0\\
        0 & 0 & D_{33}
    \end{pmatrix} \\
    \mathbf{I}_\mathrm{orth} &= \left(
    \begin{array}{ccc|ccc|ccc}
        0 & 0 & 0 & 0 & I_{131} & 0 & 0 & I_{113} & 0 \\
        0 & 0 & 0 & I_{223} & 0 & 0 & I_{232} & 0 & 0 \\
        I_{311} & I_{322} & I_{333} & 0 & 0 & 0 & 0 & 0 & 0 \\
    \end{array} \right)
\end{align}

for the point group \textit{mm}2 \cite{Authier2013a}. For easier illustration, the dipole-quadrupole tensor is represented as three \(3 \times 3\) matrices. As discussed above, in the experiment only the relative value of the components of the tensors are important because the tensor can only be determined up to any complex number. 

%\tableofcontents
\begin{figure*}%[b]
\includegraphics{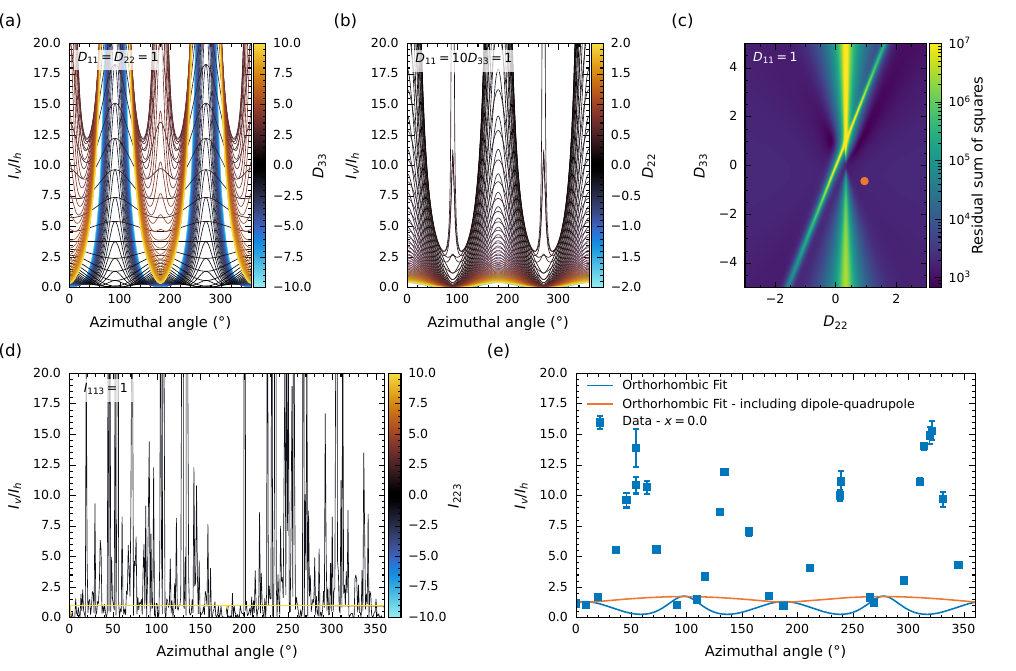}% Here is how to import EPS art
\caption{\label{Fig:OrthSim} (a)-(b),(d) Azimuthal dependence of the I-CDW scattering signal for different (a)-(b) dipole-dipole and (d) dipole-quadrupole parameters in the orthorhombic symmetry. (c) Residual sum of squares for different dipole-dipole parameters in the orthorhombic symmetry. The orange dot represents the position obtained by a fit. (e) Fits of the I-CDW scattering signal measured on sample 1 with orthorhombic symmetry. Fits with only the dipole terms and also fit including the dipole-quadrupole terms are included.}
\end{figure*}

For such a small orthorhombicity as observed in \bnap a natural assumption would be \(D_{11} \approx D_{22}\). A fit only including the dipole-dipole terms does not give satisfying results. For the majority of the parameter space, only two peaks (at \ang{90} and \ang{270}) exist. This is shown in \cref{Fig:OrthSim}a,b for a series of parameter combinations. Only for a small parameter set four peaks are reproduced, but they are shifted by \ang{45} with respect to the experimental data. Such a large misalignment can be confidently excluded using the pictures taken at each azimuth (\mbox{UE46 PGM}), the high precision of the four-circle diffractometer (ID32) and the alignment of the Bragg peak. Accordingly, the experimental data cannot be described with an orthorhombic local Ni symmetry and only dipole-dipole terms. Note that for all orthorhombic point groups, the dipole-dipole tensor has the same shape.

One possibility would be that we need to include dipole-quadrupole terms as they are allowed for the \textit{mm}2 symmetry.  Using \cref{Eq:TensorAtomicFormMulipol}, the wave vectors defined in \cref{Eq:WVDef} and including the symmetry \(I_{jkl} = I_{jlk}\) for charge scattering, the resonant tensor atomic form factor  \(\mathbf{f}^\mathrm{res}\) with the dipole-dipole and dipole-quadrupole components is given by
\begin{equation}
    \mathbf{f}_\mathrm{DD+DQ}^\mathrm{res} = \frac{i}{2} \begin{pmatrix}
        D_{11} & 0 & (-I_{113} + I_{311}) \sin(\alpha)\sin(\varphi)\\
        0 & D_{22} & (-I_{223} - I_{322}) \cos(\alpha)\\
        (I_{113} - I_{311}) \sin(\alpha)\sin(\varphi) & (-I_{223} - I_{322}) \cos(\alpha) & D_{33}
    \end{pmatrix} \ .
\end{equation}

This can be further simplified by setting \(I_{311} = I_{322} = 0\) without changing the fit results, as only the combination of \(I_{113}-I_{311}\) and \(I_{223}+I_{322}\) are relevant. The experiment is blind to the other allowed parameters and therefore they can also be neglected. As shown in \cref{Fig:OrthSim}d, the dipole-quadrupole components do not generate reasonable additions to the azimuthal dependence. Accordingly, the fits in \cref{Fig:OrthSim}e with only dipole-dipole and dipole-dipole+dipole-quadrupole components are unsatisfactory. Moreover, this discrepancy is not due to missing the right parameters, as shown by the brute-force calculated residual sum of squares (RSS) for a large parameter space presented in \cref{Fig:OrthSim}c.

One possibility would be to consider quadrupole-quadrupole interactions. However, the 4\textsuperscript{th}-rank quadrupole-quadrupole tensor has 21 independent components \cite{Authier2013a} for orthorhombic symmetry. The number of free components can be reduced by considering the symmetry of the tensor, but still too many free parameters remain to get reliable results. Moreover, the quadrupole-quadrupole interaction is commonly too weak to have such a strong influence.

\subsection{I-CDW tensor atomic form factor: monoclinic symmetry}

An inspection of the raw azimuthal dependence shows that the intensity ratio roughly follows a \(\sin^2(2\varphi)\) behavior. Inspecting the dipole-dipole tensor \(\mathbf{D}\) shows that, with \(D_{13}=D_{31}=1\) and all other components 0, the intensity ratio is given by
\begin{align}
    \frac{I_v}{I_h} & = \frac{\sin^2(2\varphi)+\cos^2(\alpha)\cos^2(2\varphi)}{\cos^2(\alpha)\cos^2(2\varphi)+\cos^4(\alpha)\sin^2(2\varphi)}\ .
\end{align}

Considering \(\alpha \approx \ang{60.5}\), \(\cos^2(\alpha) \approx 0.24\) and \(\cos^4(\alpha) \approx 0.059\), this is a promising component of the tensor atomic form factor. In addition, the maximum of \(\approx 17\) and minimum of \(1\) are close to the ones observed in the experiment. The highest symmetry allowing for the \(D_{13}\) and \(D_{31}\) components is a monoclinic symmetry with the twofold axis in the \(y\)-direction. In this experiment, the \(y\) direction is parallel to the I-CDW wave vector.

In this symmetry, the dipole-dipole tensor is given by
\begin{equation}
    \mathbf{D}_\mathrm{mono} = \begin{pmatrix}
        D_{11} & 0 & D_{13}\\
        0 & D_{22} & 0\\
        D_{13} & 0 & D_{33}
    \end{pmatrix}
\end{equation}
as discussed in the main text \cite{Authier2013a}.

Considering that both the suggested orthorhombic phase and the low temperature triclinic phase exhibit a local Ni symmetry without an inversion center, it seems likely that the here suggested monoclinic (or lower) structure exhibits no inversion center. This would allow for additional dipole-quadrupole terms. For a monoclinic symmetry, the two possible non-centrosymmetric point groups are \textit{m} and 2. The third possible monoclinic point group, 2/\textit{m}, does not allow for dipole-quadrupole components as there is an inversion center. For the point group 2 with the twofold axis along the \(y\)-direction, the dipole-quadrupole tensor is given by
\begin{equation}
    \mathbf{I}_\mathrm{mono, 2} = \left(
    \begin{array}{ccc|ccc|ccc}
        0 & 0 & 0 & I_{123} & 0 & I_{112} & I_{132} & 0 & I_{121} \\
        I_{211} & I_{222} & I_{233} & 0 & I_{231} & 0 & 0 & I_{213} & 0 \\
        0 & 0  & 0 & I_{323} & 0 & I_{312} & I_{332} & 0 & I_{321} \\
    \end{array} \right) 
\end{equation}
and for the point group \textit{m} by
\begin{equation}
    \mathbf{I}_\text{mono, \textit{m}} = \left(
    \begin{array}{ccc|ccc|ccc}
        I_{111} & I_{122} & I_{133} & 0 & I_{131} & 0 & 0 & I_{113} & 0 \\
        0 & 0  & 0 & I_{223} & 0 & I_{212} & I_{232} & 0 & I_{221} \\
        I_{311} & I_{322} & I_{333} & 0 & I_{331} & 0 & 0 & I_{313} & 0 \\        
    \end{array} \right) \ .
\end{equation}

Including again the symmetry of the tensor for charge scattering, one obtains
\begin{align}
    \mathbf{f}_\mathrm{DD+DQ,2}^\mathrm{res} &= \begin{pmatrix}
        f_{11} & f_{12} & f_{13} \\
        - f_{12} &f_{22} & f_{23}\\
        f_{13} & -f_{23} & f_{33}
    \end{pmatrix} \\
    f_{11} &= D_{11} - i I_{112} \cos(\alpha)\\
    f_{12} &= \frac{i}{2} \sin(\alpha) (( I_{123} -  I_{213}) \cos(\varphi) + (- I_{112} + I_{211}) \sin(\varphi)) \\
    f_{13} &= D_{13} - \frac{i}{2} (I_{123} + 
    I_{312}) \cos(\alpha) \\
    f_{22} &= D_{22} - i I_{222} \cos(\alpha)\\
    f_{23} &= \frac{i}{2} \sin(\alpha) ((I_{233} - I_{323}) \cos(\varphi) + (- I_{213} + I_{312}) \sin(\varphi)) \\
    f_{33} &= D_{33}- i I_{323} \cos(\alpha) \ .
\end{align}
for the effective tensor atomic form factor for point group 2. This can be simplified by setting \(I_{211}=I_{233}=0\). This is possible as only the combination \(I_{112}-I_{211}\) and \(I_{323}-I_{233}\) can be measured. The other components cannot be further simplified. By fixing \(I_{312}=-1\) in this symmetry, a total of 9 free parameters exist. To account for possible misalignment, an offset is included in the fit. In order not to include further free parameters, the offset was fixed to a value obtained with \(D_{13}\) as the only non-zero parameter. Similarly to the point group 2, the tensor atomic form factor can be expressed as
\begin{align}
    \mathbf{f}_\mathrm{DD+DQ, m}^\mathrm{res} &= \begin{pmatrix}
        D_{11} & f_{12} & D_{13}+f_{13} \\
        f_{12} & D_{22} & f_{23}\\
        D_{13}-f_{13} & f_{23} & D_{33}
    \end{pmatrix} \\
    f_{12} &= - \frac{i}{2}( I_{122} + I_{212}) \cos(\alpha)\\
    f_{13} &= \frac{i}{2} \sin(\alpha) ((I_{133} - I_{313}) \cos(\varphi) + (-I_{113} + I_{311}) \sin(\varphi)) \\
    f_{23} &= - \frac{i}{2}( I_{223} + I_{322}) \cos(\alpha)
\end{align}
considering the symmetry of point group \textit{m}. Here, \(I_{212}=I_{313}=I_{113}=I_{322}=0\) can be chosen, as these components only appear in combination with other components. By fixing \(D_{13}=1\), in total, seven free parameters remain. 

Including the dipole-quadrupole Terms lower the residual sum of squares (RSS). However, there are two many free parameters, such that the actual fit is nearly arbitrary as the fit errors exceed the values by orders of magnitudes and many parameters show a high correlation in the fit. For this the exact results of dipole-quadrupole terms are not discussed and shown. For quadrupole-quadrupole Terms even more free parameters exist, which make an further analysis of them also pointless.

For the C-CDW the discussion is equivalent. However, the polarization vectors \(\vec{\epsilon}\) and the wave vectors \(\vec{k}\) must be rotated with the rotation matrix \(\mathbf{R}\) due to the changed scattering geometry involving the additional tilt of \(\approx \ang{19.5}\). Within the triclinic phase the local point group of the Nickel atom is \(1\). Hence, dipole-quadrupole terms are allowed and in the tensor all components are possible. For this reason an discussion of the dipole-quadrupole terms is not sensible even though they improve the RSS significantly.

\section{Fit results and procedure} 

\label{sec:FitPro}

\begin{table}
    \centering
    \caption{\label{Tab:FitsSM} Fitted dipole-dipole tensor for the azimuthal dependence of the I-CDW and C-CDW in the \(x=0.0\) and \(x\approx 0.059\) samples. Only the by symmetry allowed components are given, and the symmetry of the dipole-dipole tensor is included. In addition the fitted azimuthal offset \(\Delta\varphi\) is stated.}
    \begin{tabular}{l c c}
      & \(\mathbf{D}\) &  \(\Delta \varphi\) \\
    \hline
    \makecell{I-CDW\\\(x=0.0\)} & 
    \(\begin{pmatrix}
        0.000(20) & \  & 1 \\
         \ &0.020(20) & \ \\ 
       1 & \ & 0.010(20) 
    \end{pmatrix}\)
        &  \ang{-7.5(4)}\\
    \makecell{C-CDW\\\(x=0.0\)} &        
        \(\begin{pmatrix} 
        -0.06(6) & -0.060(20) & 1 \\
        -0.060(20) & -0.16(8) & -0.01(3)\\ 
       1 & -0.01(3) & -0.19(8) 
        \end{pmatrix}\) & \ang{0.6(14)} \\
        \makecell{I-CDW\\\(x\approx0.059\)} & 
    \(\begin{pmatrix}
        -0.070(20) & \  & 1 \\
         \ & -0.100(20) & \ \\ 
       1 & \ & -0.07(3) 
    \end{pmatrix}\)
        &  \ang{-111.6(5)}\\
    \end{tabular}
\end{table}

In order to fit the azimuthal dependence the dominating component \(D_{13}\) was fixed to 1, as within \cref{ed:IntRatioFull} the tensor atomic form factor can be only determined up to a complex number. To account for a potential offset or misalignment of the sample, an azimuthal offset \(\Delta\varphi\) was determined by fitting the offset and only keeping \(D_{13}=1\) as only non-zero component of the tensor atomic form factor. In a second step the fit off the full dipole-dipole tensor \(\mathbf{D}\) was performed by adding all other by symmetry allowed components and keep \(\Delta\varphi\) at the previously found value. To cross check the results with the linear polarization dependencies, the obtained dipole-dipole tensor \(\mathbf{D}\) was used to calculate the absolute intensity change and then scaled to fit the measured intensities.

The obtained fit parameters are presented in \cref{Tab:FitsSM}. Note that the offset for the \(x\approx0.059\) sample is this large, as during the mounting the sample was offset on purpose by \ang{110} to compensate for the limited and asymmetric moving range of the motor.

\FloatBarrier
\section{Temperature dependence of the I-CDW in resonance}

To check of a potentially different temperature dependence of the orbital order related to the I-CDW a temperature dependence of the scattering signal at the resonance of the I-CDW was measured. The measured raw \(\theta-2\theta\)-scans and the integrated intensity versus temperature are shown in \cref{Fig:TDep}. We could not detect a significant different temperature dependence of the scattering signal at the Ni-resonance compared to the measurements with hard X-Rays \cite{Lacmann2025,Yao2022}.

%\tableofcontents
\begin{figure*}%[b]
\includegraphics{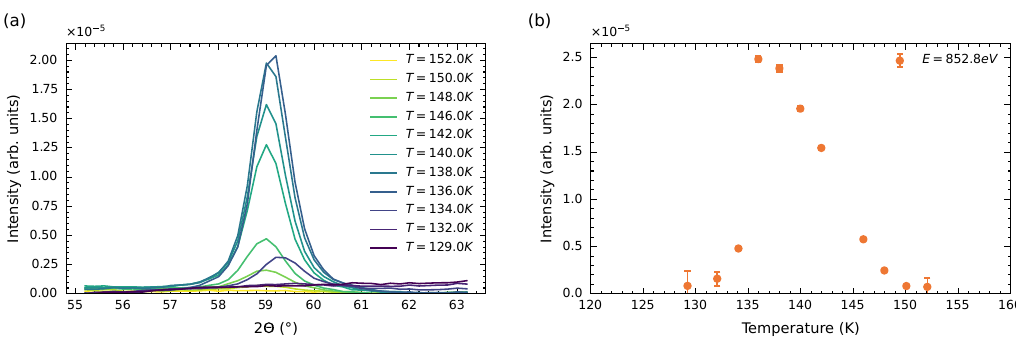}% Here is how to import EPS art
\caption{\label{Fig:TDep}(a) \(\theta-2\theta\)-scans of the I-CDW at \((0\ 0.28\ 0)\) for different temperatures. (b) Integrated temperature of the I-CDW versus temperature. The measurements were performed for a \(x=0.0\) sample.}
\end{figure*}

\FloatBarrier
\section{Linear polarization dependence of the scattering signal}

As mentioned in the main text and above, in addition to the azimuthal dependence at selected azimuths also a full incoming linear polarization dependence was performed to cross check the obtained tensor atomic form factor. This was done for both the I-CDW and the C-CDW for the \(x=0.0\) sample. The measured \(\theta-2\theta\)-scans for each azimuth and the integrated intensities, including the fits are shown in \cref{Fig:LinPolICDW} and \cref{Fig:LinPolCCDW} for the I-CDW and C-CDW respectively. The fits were obtained as described before.

\begin{figure*}%[b]
\includegraphics{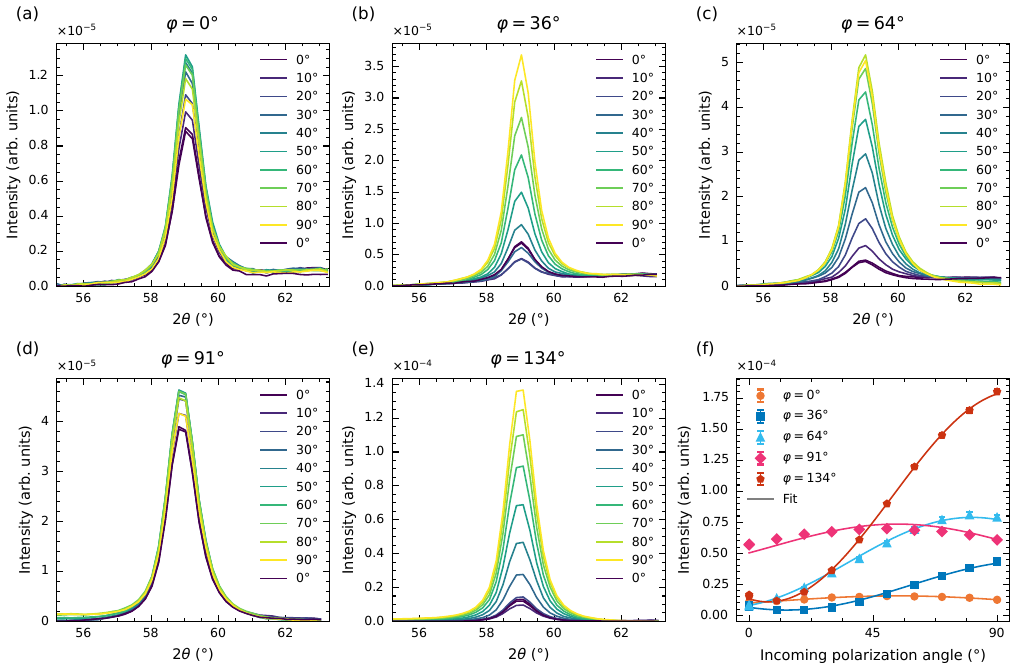}% Here is how to import EPS art
\caption{\label{Fig:LinPolICDW} (a)-(e) \(\theta-2\theta\)-scans of the I-CDW for different incoming linear polarizations at different azimuths --- (a) \ang{0}, (b) \ang{36}, (c) \ang{64}, (d) \ang{91} and (e) \ang{134}. (f) Integrated intensity versus incoming linear polarization for the different azimuthal rotations. In addition the with tensor atomic form factor calculated intensity dependence is shown. The measurements are for the \(x=0.0\) sample. }
\end{figure*}

\begin{figure*}%[b]
\includegraphics{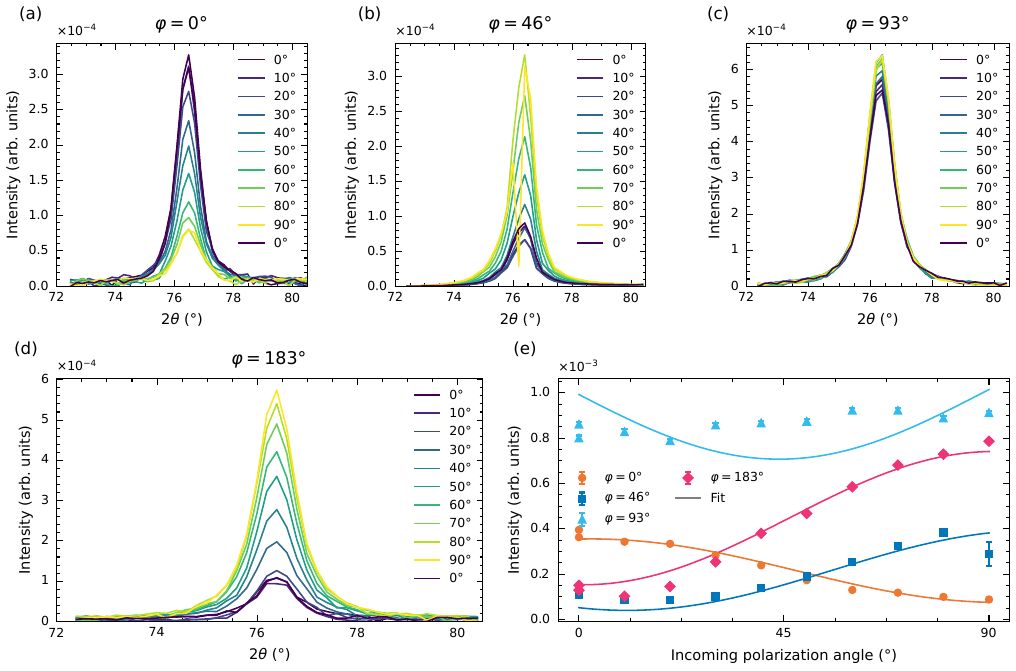}% Here is how to import EPS art
\caption{\label{Fig:LinPolCCDW} (a)-(e) \(\theta-2\theta\)-scans of the C-CDW for different incoming linear polarizations at different azimuths --- (a) \ang{0}, (b) \ang{46}, (c) \ang{93} and (d) \ang{93}. (f) Integrated intensity versus incoming linear polarization for the different azimuthal rotations. In addition the with tensor atomic form factor calculated intensity dependence is shown. The measurements are for the \(x=0.0\) sample.}
\end{figure*}

\FloatBarrier
\section{Energy dependence of the scattering signal}

In addition to the energy dependence presented in the main text further energy dependencies and also total electron yield (TEY) representing the x-ray absorption were measured. These additional measurements generally agree well with the measurements in the main text and are presented in \cref{fig:Sup3}.

\begin{figure*}%[b]
\includegraphics{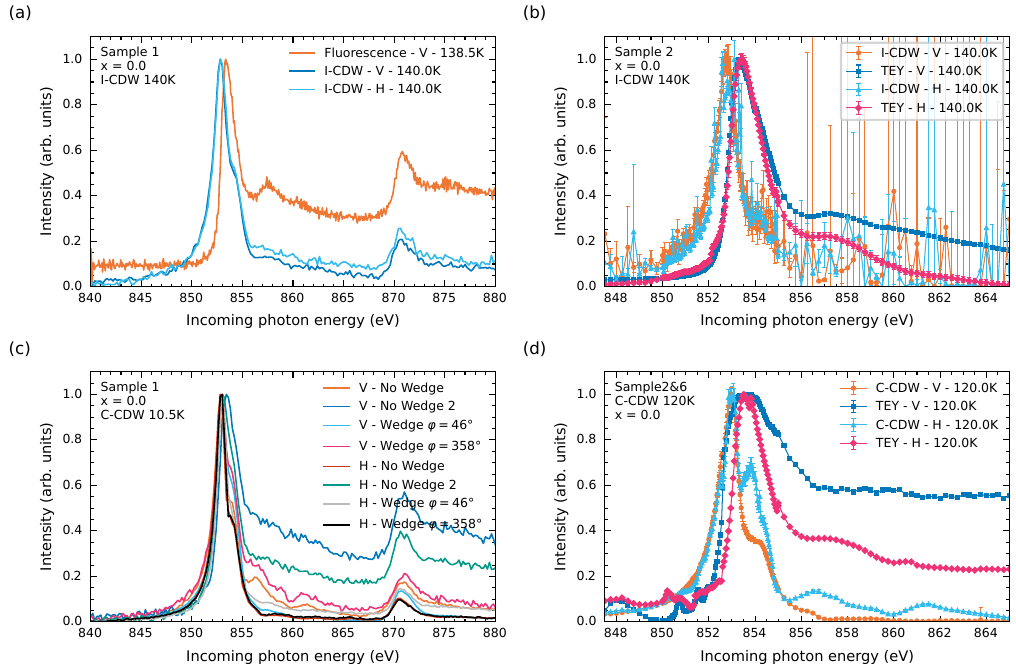}% Here is how to import EPS art
\caption{\label{fig:Sup3} (a)-(b) Energy dependence of the scattering signal at the I-CDW position, TEY or fluoresence at \qty{140}{\kelvin} measured on (a) sample 1 and (b) sample 2. (c)-(d) Energy dependence of the scattering signal at the C-CDW position or TEY at (c) \qty{10.5}{\kelvin} measured on sample 1 and (d) \qty{120}{\kelvin} measured on sample 2 and 6 . For the C-CDW measurements different orientations of the sample are shown.}
\end{figure*}

\FloatBarrier
\section{RIXS measurements at the I-CDW and C-CDW position}

\begin{figure*}%[b]
\includegraphics{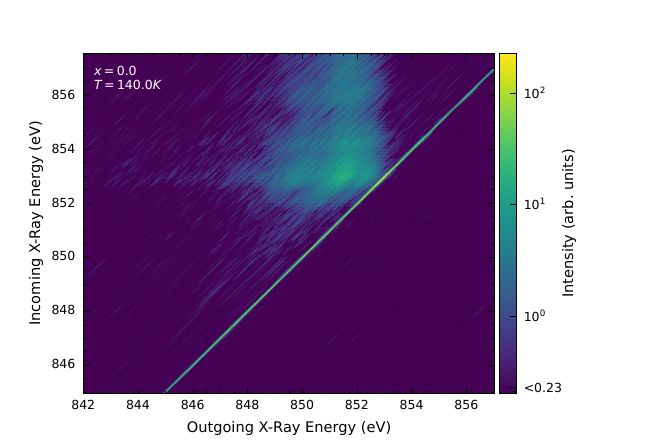}% Here is how to import EPS art
\caption{\label{fig:RIXSEDep} Incoming and outgoing energy dependence at the I-CDW position. The measurements were performed at sample 2.}
\end{figure*}

As mentioned in the main text also RIXS measurements were performed. The incoming photon energy dependence shown in \cref{fig:RIXSEDep}. In this dependence no relevant inelastic signal could be observed. Only strong x-ray fluorescence --- shows up as intensity with constant outgoing x-ray energy ---  and the elastic line could be observed at the I-CDW position. This also confirmed by the \(q\) dependent measurements shown in \cref{fig:Sup4}, which does not show a significant change of the inelastic signal through the I-CDW and C-CDW positions.

\begin{figure*}%[b]
\includegraphics{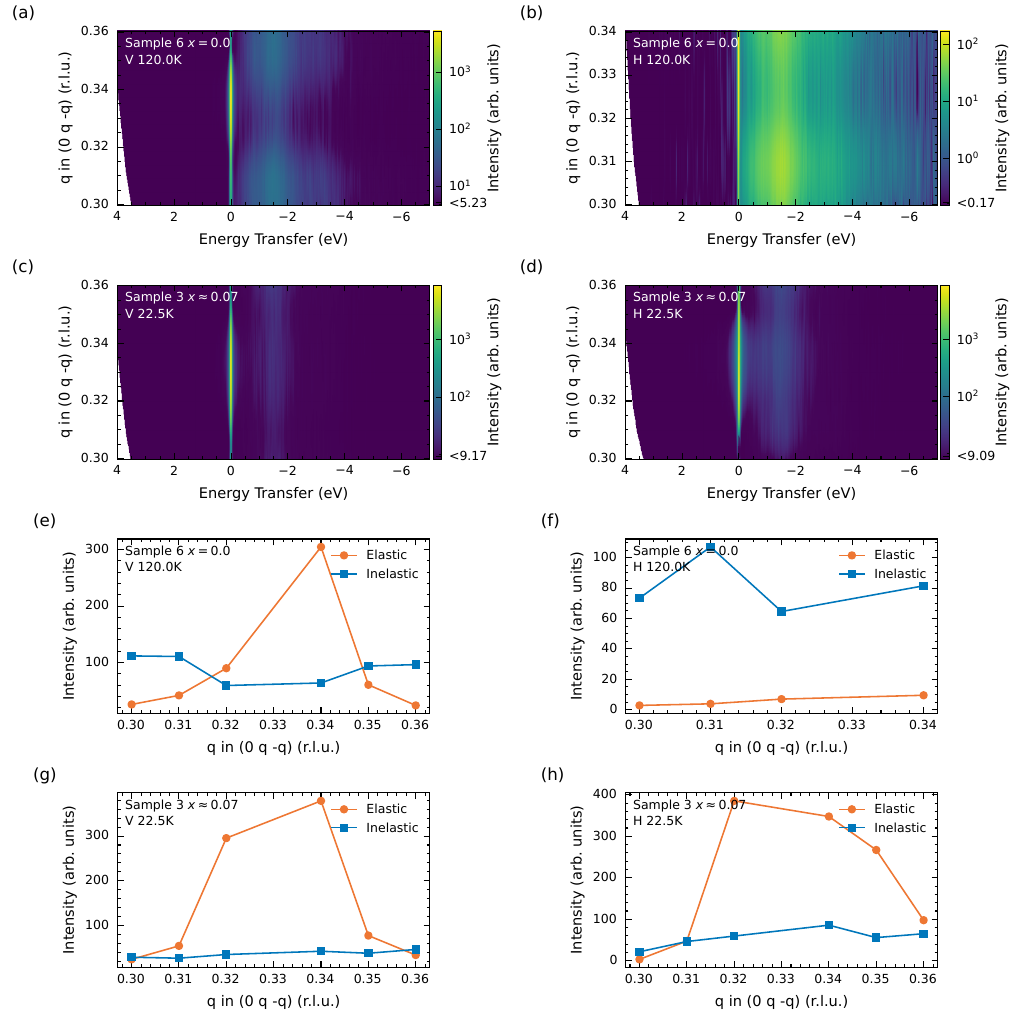}% Here is how to import EPS art
\caption{\label{fig:Sup4} (a)-(d) Intensity maps of the RIXS signal for different positions around the C-CDW measured at (a),(b) \qty{120}{\kelvin} on sample 6 with incoming vertical and horizontal polarization and (c),(d) \qty{22.5}{\kelvin} on sample 3 with incoming vertical and horizontal polarization, respectively. (e)-(h) Integrated intensity of the elastic and inelastic signal of the colormaps in (a)-(d).}
\end{figure*}

\FloatBarrier
\section{REXS measurements around (0 0.28 1)}

At the nickel resonance there are two positions of the I-CDW --- \((0\ 0.28\ 0)\) and \((0\ 0.28\ 1)\)  --- which lie within the possible momentum transfer. From the scattering geometry the position at is \((0\ 0.28\ 1)\) would be favorable, as this would not requiring measuring on the side of the sample, but allows for measurements on the larger and much smoother surface of the plate-like samples. However, in hard X-ray measurements this peak is a forbidden peak. Nonetheless, this does not fully exclude that the peak could not be observed in resonance. However, we could not observe any scattering signal at \((0\ 0.28\ 1)\). This is independent of the fact that the sample is in air cleaved or cleaved in vacuum. The relevant scans which show the absence of any intensity at this position are shown in \cref{fig:Sup6}. 

\begin{figure*}%[b]
\includegraphics{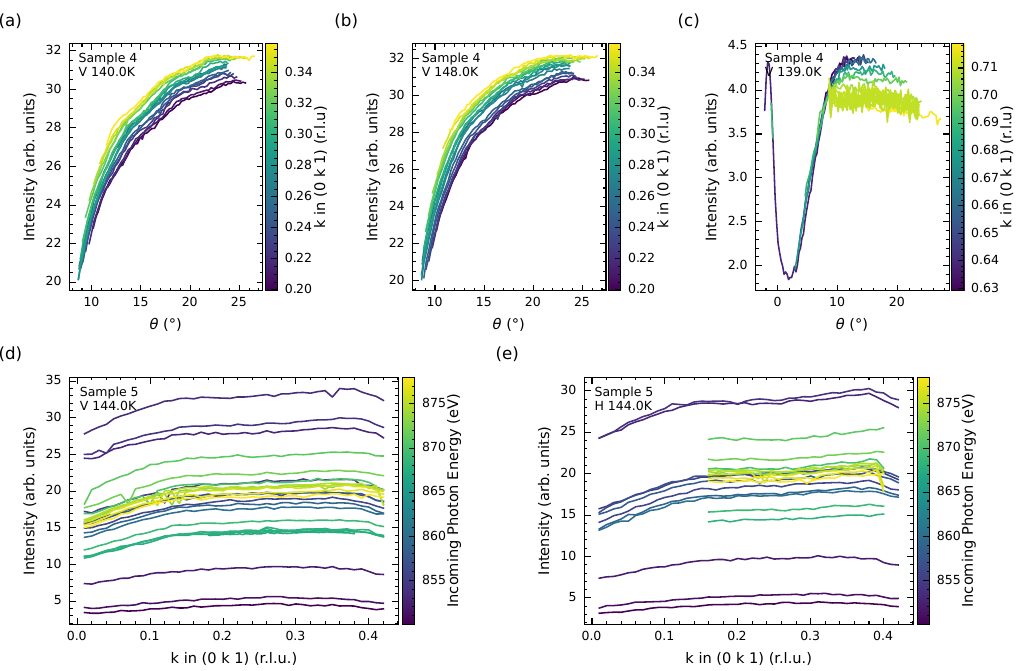}% Here is how to import EPS art
\caption{\label{fig:Sup6} (a)-(c) \(\theta-2\theta\) scans around the \((0\ 0.28\ 1)\) position for different values of \(k\) at (a) \qty{140}{\kelvin}, (b) \qty{148}{\kelvin} and (c) (a) \qty{139}{\kelvin}. The measurements were performed on sample 4. (d),(e) Scans along the \(k\)-directions around \((0\ 0.28\ 1)\) position for different incoming photon energies at \qty{144}{\kelvin} with (d) incoming vertical polarization and (e) incoming horizontal polarization. Measurements were performed on sample 5.}
\end{figure*}

\bibliography{REXS2024}% Produces the bibliography via BibTeX.

\end{document}
